# Supplementary material for: Read-only Prompt Optimization for Vision-Language Few-shot Learning
Source: arXiv:2308.14960 source file (2023-11-10)
Supplement: Supplementary file 1 [file supple_tab1.tex]

\begin{table*}[t]
  % \caption{\textbf{abbab.}
  % \centering
% \setlength{\tabcolsep}{6pt}
    % abcd
  % }
\caption{\textbf{Ablation on our components in base to new generalization setting.} We evaluate base to new generalization performance by ablating read-only mask and special initialization.}
  \begin{subtable}{0.3\linewidth}
  \centering
  \caption{Average over 11 datasets}
  \begin{tabular}{l|c|c|c}
    \toprule
    Methods & Base & Novel & H\\
    \midrule
    w.o mask & \textcolor{DarkGray}{79.97} & \textcolor{DarkGray}{69.90} & 74.02 \\
    w.o init & \textcolor{DarkGray}{82.27} & \textcolor{DarkGray}{72.78} & 76.78 \\
    RPO    &   \textcolor{DarkGray}{81.13}    &   \textcolor{DarkGray}{75.00}    &   \textbf{77.78} \\
    
    \bottomrule
    \end{tabular}
    \label{tab:9.a}
  \end{subtable}
  \hfill
  \begin{subtable}{0.3\linewidth}
  \centering
  \caption{ImageNet.}
  \begin{tabular}{l|c|c|c}
    \toprule
    Methods & Base & Novel & H\\
    \midrule
    w.o mask & \textcolor{DarkGray}{76.10} & \textcolor{DarkGray}{69.03} & 72.40 \\
    w.o init & \textcolor{DarkGray}{76.57} & \textcolor{DarkGray}{70.57} & 73.45 \\
    RPO    &   \textcolor{DarkGray}{76.60}    &   \textcolor{DarkGray}{71.57}    &   \textbf{74.00} \\
    
    \bottomrule
  \end{tabular}
  \label{tab:9.b}
  \end{subtable}
  \hfill
  \begin{subtable}{0.3\linewidth}
  \centering
  \caption{Caltech101.}
  \begin{tabular}{l|c|c|c}
    \toprule
    Methods & Base & Novel & H\\
    \midrule
    w.o mask & \textcolor{DarkGray}{98.10} & \textcolor{DarkGray}{92.87} & 95.41 \\
    w.o init & \textcolor{DarkGray}{98.60} & \textcolor{DarkGray}{92.47} & 95.43 \\
    RPO    &   \textcolor{DarkGray}{97.97}    &   \textcolor{DarkGray}{94.37}    &   \textbf{96.03} \\
    \bottomrule
  \end{tabular}
  \label{tab:9.c}
  \end{subtable}
  \hfill
  \vspace{0.5em}
  \begin{subtable}{0.3\linewidth}
  \centering
  \caption{OxfordPets.}
  \begin{tabular}{l|c|c|c}
    \toprule
    Methods & Base & Novel & H\\
    \midrule
    w.o mask & \textcolor{DarkGray}{95.13} & \textcolor{DarkGray}{96.77} & 95.95 \\
    w.o init & \textcolor{DarkGray}{95.57} & \textcolor{DarkGray}{96.90} & \textbf{96.23} \\
    RPO    &   \textcolor{DarkGray}{94.63}    &   \textcolor{DarkGray}{97.50}    &  96.05 \\
    \bottomrule
  \end{tabular}
  \label{tab:9.d}
  \end{subtable}
  \hfill
  \begin{subtable}{0.3\linewidth}
  \centering
  \caption{StanfordCars.}
  \begin{tabular}{l|c|c|c}
    \toprule
    Methods & Base & Novel & H\\
    \midrule
    w.o mask & \textcolor{DarkGray}{74.53} & \textcolor{DarkGray}{71.47} & 72.96 \\
    w.o init & \textcolor{DarkGray}{72.93} & \textcolor{DarkGray}{73.33} & 73.13 \\
    RPO    &   \textcolor{DarkGray}{73.87}    &   \textcolor{DarkGray}{75.53}    &   \textbf{74.69} \\
    \bottomrule
  \end{tabular}
  \label{tab:9.e}
  \end{subtable}
  \hfill
  \begin{subtable}{0.3\linewidth}
  \centering
  \caption{Flowers102.}
  \begin{tabular}{l|c|c|c}
    \toprule
    Methods & Base & Novel & H\\
    \midrule
    w.o mask & \textcolor{DarkGray}{96.87} & \textcolor{DarkGray}{71.47} & 82.92 \\
    w.o init & \textcolor{DarkGray}{94.70} & \textcolor{DarkGray}{74.83} & 83.60 \\
    RPO    &   \textcolor{DarkGray}{94.13}    &   \textcolor{DarkGray}{76.67}    &   \textbf{84.50} \\
    \bottomrule
  \end{tabular}
  \label{tab:9.f}
  \end{subtable}
  \hfill
  \vspace{0.5em}
  \begin{subtable}{0.3\linewidth}
  \centering
  \caption{Food101.}
  \begin{tabular}{l|c|c|c}
    \toprule
    Methods & Base & Novel & H\\
    \midrule
    w.o mask & \textcolor{DarkGray}{88.97} & \textcolor{DarkGray}{88.73} & 88.85 \\
    w.o init & \textcolor{DarkGray}{90.23} & \textcolor{DarkGray}{89.87} & 90.05 \\
    RPO    &   \textcolor{DarkGray}{90.33}    &   \textcolor{DarkGray}{90.83}    &   \textbf{90.58} \\
    \bottomrule
  \end{tabular}
  \label{tab:9.g}
  \end{subtable}
  \hfill
  \begin{subtable}{0.3\linewidth}
  \centering
  \caption{FGVCAircraft.}
  \begin{tabular}{l|c|c|c}
    \toprule
    Methods & Base & Novel & H\\
    \midrule
    w.o mask & \textcolor{DarkGray}{35.53} & \textcolor{DarkGray}{29.90} & 32.45 \\
    w.o init & \textcolor{DarkGray}{38.37} & \textcolor{DarkGray}{31.43} & 34.55 \\
    RPO    &   \textcolor{DarkGray}{37.33}    &   \textcolor{DarkGray}{34.20}    &   \textbf{35.70} \\
    \bottomrule
  \end{tabular}
  \label{tab:9.h}
  \end{subtable}
  \hfill
  \begin{subtable}{0.3\linewidth}
  \centering
  \caption{SUN397.}
  \begin{tabular}{l|c|c|c}
    \toprule
    Methods & Base & Novel & H\\
    \midrule
    w.o mask & \textcolor{DarkGray}{78.96} & \textcolor{DarkGray}{76.10} & 77.50 \\
    w.o init & \textcolor{DarkGray}{80.53} & \textcolor{DarkGray}{77.60} & 79.04 \\
    RPO    &   \textcolor{DarkGray}{80.60}    &   \textcolor{DarkGray}{77.80}    &   \textbf{79.18} \\
    \bottomrule
  \end{tabular}
  \label{tab:9.i}
  \end{subtable}
  \hfill
  \vspace{0.5em}
  \begin{subtable}{0.3\linewidth}
  \centering
  \caption{DTD.}
  \begin{tabular}{l|c|c|c}
    \toprule
    Methods & Base & Novel & H\\
    \midrule
    w.o mask & \textcolor{DarkGray}{78.67} & \textcolor{DarkGray}{55.77} & 65.25 \\
    w.o init & \textcolor{DarkGray}{79.93} & \textcolor{DarkGray}{63.13} & \textbf{70.53} \\
    RPO    &   \textcolor{DarkGray}{76.70}    &   \textcolor{DarkGray}{62.13}    &  68.61 \\
    \bottomrule
  \end{tabular}
  \label{tab:9.j}
  \end{subtable}
  \hfill
  \begin{subtable}{0.3\linewidth}
  \centering
  \caption{EuroSAT.}
  \begin{tabular}{l|c|c|c}
    \toprule
    Methods & Base & Novel & H\\
    \midrule
    w.o mask & \textcolor{DarkGray}{74.70} & \textcolor{DarkGray}{45.13} & 54.57 \\
    w.o init & \textcolor{DarkGray}{93.80} & \textcolor{DarkGray}{55.13} & 69.37 \\
    RPO    &   \textcolor{DarkGray}{86.63}    &   \textcolor{DarkGray}{68.97}    &   \textbf{76.79} \\
    \bottomrule
  \end{tabular}
  \label{tab:9.k}
  \end{subtable}
  \hfill
  \vspace{0.5em}
  \begin{subtable}{0.3\linewidth}
  \centering
  \caption{UCF101.}
  \begin{tabular}{l|c|c|c}
    \toprule
    Methods & Base & Novel & H\\
    \midrule
    w.o mask & \textcolor{DarkGray}{82.07} & \textcolor{DarkGray}{70.63} & 75.92 \\
    w.o init & \textcolor{DarkGray}{83.77} & \textcolor{DarkGray}{75.27} & 79.29 \\
    RPO    &   \textcolor{DarkGray}{83.67}    &   \textcolor{DarkGray}{75.43}    &   \textbf{79.34} \\
    \bottomrule
  \end{tabular}
  \label{tab:9.l}
  \end{subtable}
  \hfill
  \vspace{0.5em}
\label{tab:ablation_11}
\end{table*}
