# Supplementary material for: Read-only Prompt Optimization for Vision-Language Few-shot Learning
Source: arXiv:2308.14960 source file (2023-11-10)
Supplement: Supplementary file 2 [file supple_tab2.tex]

\begin{table*}[h]
  % \caption{\textbf{abbab.}
  % \centering
% \setlength{\tabcolsep}{6pt}
    % abcd
  % }
\caption{\textbf{Comparison of CoCoOp, vis-RPO, text-RPO and RPO in the Base to new generalization setting.} We evaluate base to new generalization performance with unimodal RPO trained with 16-shot sampled training data.}
  \begin{subtable}{0.3\linewidth}
  \centering
  \caption{Average over 11 datasets}
  \begin{tabular}{l|c|c|c}
    \toprule
    Methods & Base & Novel & H\\
    \midrule
    CoCoOp  &   \textcolor{DarkGray}{80.47}   &   \textcolor{DarkGray}{71.69}   &  75.83  \\
    \midrule
    text-RPO & \textcolor{DarkGray}{79.54} & \textcolor{DarkGray}{74.83} & 77.01 \\
    RPO    &   \textcolor{DarkGray}{81.13}    &   \textcolor{DarkGray}{75.00}    &   \textbf{77.78} \\
    \bottomrule
    \end{tabular}
    \label{tab:11.a}
  \end{subtable}
  \hfill
  \begin{subtable}{0.3\linewidth}
  \centering
  \caption{ImageNet.}
  \begin{tabular}{l|c|c|c}
    \toprule
    Methods & Base & Novel & H\\
    \midrule
    CoCoOp  &   \textcolor{DarkGray}{75.98}   &   \textcolor{DarkGray}{70.43}   &   73.10 \\
    \midrule
    text-RPO & \textcolor{DarkGray}{76.13} & \textcolor{DarkGray}{70.70} & 73.31 \\
    RPO    &   \textcolor{DarkGray}{76.60}    &   \textcolor{DarkGray}{71.57}    &   \textbf{74.00} \\
    \bottomrule
  \end{tabular}
  \label{tab:11.b}
  \end{subtable}
  \hfill
  \begin{subtable}{0.3\linewidth}
  \centering
  \caption{Caltech101.}
  \begin{tabular}{l|c|c|c}
    \toprule
    Methods & Base & Novel & H\\
    \midrule
    CoCoOp  &   \textcolor{DarkGray}{97.96}   &   \textcolor{DarkGray}{93.81}   &  95.84  \\
    \midrule
    text-RPO & \textcolor{DarkGray}{97.76} & \textcolor{DarkGray}{93.96} & 95.82 \\
    RPO    &   \textcolor{DarkGray}{97.97}    &   \textcolor{DarkGray}{94.37}    &  \textbf{96.03}  \\
    \bottomrule
  \end{tabular}
  \label{tab:11.c}
  \end{subtable}
  \hfill
  \vspace{0.5em}
  \begin{subtable}{0.3\linewidth}
  \centering
  \caption{OxfordPets.}
  \begin{tabular}{l|c|c|c}
    \toprule
    Methods & Base & Novel & H\\
    \midrule
    CoCoOp  &   \textcolor{DarkGray}{95.20}   &   \textcolor{DarkGray}{97.69}   &  \textbf{96.43} \\
    \midrule
    text-RPO & \textcolor{DarkGray}{94.56} & \textcolor{DarkGray}{97.16} & 95.84 \\
    RPO    &   \textcolor{DarkGray}{94.63}    &   \textcolor{DarkGray}{97.50}    &   96.05 \\
    \bottomrule
  \end{tabular}
  \label{tab:11.d}
  \end{subtable}
  \hfill
  \begin{subtable}{0.3\linewidth}
  \centering
  \caption{StanfordCars.}
  \begin{tabular}{l|c|c|c}
    \toprule
    Methods & Base & Novel & H \\
    \midrule
    CoCoOp  &   \textcolor{DarkGray}{70.49}  &   \textcolor{DarkGray}{73.59}   &   72.01 \\
    \midrule
    text-RPO & \textcolor{DarkGray}{72.16} & \textcolor{DarkGray}{74.4} & 73.26 \\
    RPO    &   \textcolor{DarkGray}{73.87}    &   \textcolor{DarkGray}{75.53}    &  \textbf{74.69}  \\
    \bottomrule
  \end{tabular}
  \label{tab:11.e}
  \end{subtable}
  \hfill
  \begin{subtable}{0.3\linewidth}
  \centering
  \caption{Flowers102.}
  \begin{tabular}{l|c|c|c}
    \toprule
    Methods & Base & Novel & H\\
    \midrule
    CoCoOp  &   \textcolor{DarkGray}{94.87}   &   \textcolor{DarkGray}{71.75}   &   81.71 \\
    \midrule
    text-RPO & \textcolor{DarkGray}{91.70} & \textcolor{DarkGray}{74.90} & 82.45 \\
    RPO    &   \textcolor{DarkGray}{94.13}    &   \textcolor{DarkGray}{76.67}    &   \textbf{84.50} \\
    \bottomrule
  \end{tabular}
  \label{tab:11.f}
  \end{subtable}
  \hfill
  \vspace{0.5em}
  \begin{subtable}{0.3\linewidth}
  \centering
  \caption{Food101.}
  \begin{tabular}{l|c|c|c}
    \toprule
    Methods & Base & Novel & H\\
    \midrule
    CoCoOp  &   \textcolor{DarkGray}{90.70}   &   \textcolor{DarkGray}{91.29}   &   \textbf{90.99} \\
    \midrule
    text-RPO & \textcolor{DarkGray}{89.90} & \textcolor{DarkGray}{90.06} & 89.98 \\
    RPO    &   \textcolor{DarkGray}{90.33}    &   \textcolor{DarkGray}{90.83}    &   90.58
 \\
    \bottomrule
  \end{tabular}
  \label{tab:11.g}
  \end{subtable}
  \hfill
  \begin{subtable}{0.3\linewidth}
  \centering
  \caption{FGVCAircraft.}
  \begin{tabular}{l|c|c|c}
    \toprule
    Methods & Base & Novel & H\\
    \midrule
    CoCoOp  &   \textcolor{DarkGray}{33.41}   &   \textcolor{DarkGray}{23.71}   &   27.74 \\
    \midrule
    text-RPO & \textcolor{DarkGray}{36.5} & \textcolor{DarkGray}{35.7} & \textbf{36.09} \\
    RPO    &   \textcolor{DarkGray}{37.33}    &   \textcolor{DarkGray}{34.20}    &  35.70  \\
    \bottomrule
  \end{tabular}
  \label{tab:11.h}
  \end{subtable}
  \hfill
  \begin{subtable}{0.3\linewidth}
  \centering
  \caption{SUN397.}
  \begin{tabular}{l|c|c|c}
    \toprule
    Methods & Base & Novel & H\\
    \midrule
    CoCoOp  &   \textcolor{DarkGray}{79.74}   &   \textcolor{DarkGray}{76.86}   &   78.27 \\
    \midrule
    text-RPO & \textcolor{DarkGray}{79.56} & \textcolor{DarkGray}{77.03} & 78.27 \\
    RPO    &   \textcolor{DarkGray}{80.60}    &   \textcolor{DarkGray}{77.80}    &   \textbf{79.18} \\
    \bottomrule
  \end{tabular}
  \label{tab:11.i}
  \end{subtable}
  \hfill
  \vspace{0.5em}
  \begin{subtable}{0.3\linewidth}
  \centering
  \caption{DTD.}
  \begin{tabular}{l|c|c|c}
    \toprule
    Methods & Base & Novel & H\\
    \midrule
    CoCoOp  &   \textcolor{DarkGray}{77.01}   &   \textcolor{DarkGray}{56.00}   &   64.85 \\
    \midrule
    text-RPO & \textcolor{DarkGray}{75.06} & \textcolor{DarkGray}{62.60} & 68.26 \\
    RPO    &   \textcolor{DarkGray}{76.70}    &   \textcolor{DarkGray}{62.13}    &  \textbf{68.61} \\
    \bottomrule
  \end{tabular}
  \label{tab:11.j}
  \end{subtable}
  \hfill
  \begin{subtable}{0.3\linewidth}
  \centering
  \caption{EuroSAT.}
  \begin{tabular}{l|c|c|c}
    \toprule
    Methods & Base & Novel & H\\
    \midrule
    CoCoOp  &   \textcolor{DarkGray}{87.49}   &   \textcolor{DarkGray}{60.04}   &   71.21 \\
    \midrule
    text-RPO & \textcolor{DarkGray}{79.90} & \textcolor{DarkGray}{71.60} & 75.52 \\
    RPO    &   \textcolor{DarkGray}{86.63}    &   \textcolor{DarkGray}{68.97}    &   \textbf{76.79} \\
    \bottomrule
  \end{tabular}
  \label{tab:11.k}
  \end{subtable}
  \hfill
  %\vspace{0.5em}
  \begin{subtable}{0.3\linewidth}
  \centering
  \caption{UCF101.}
  \begin{tabular}{l|c|c|c}
    \toprule
    Methods & Base & Novel & H\\
    \midrule
    CoCoOp  &   \textcolor{DarkGray}{82.33}   &   \textcolor{DarkGray}{73.45}   &   77.64 \\
    \midrule
    text-RPO & \textcolor{DarkGray}{81.70} & \textcolor{DarkGray}{75.1} & 78.26 \\
    RPO    &   \textcolor{DarkGray}{83.67}    &   \textcolor{DarkGray}{75.43}    &   \textbf{79.34} \\
    \bottomrule
  \end{tabular}
  \label{tab:11.l}
  \end{subtable}
  \hfill
  \vspace{0.5em}
\label{tab:uni_rpo_11}
\end{table*}
