# Supplementary material for: Read-only Prompt Optimization for Vision-Language Few-shot Learning
Source: arXiv:2308.14960 source file (2023-11-10)
Supplement: Supplementary file 3 [file supple_tab3.tex]

\begin{table*}[t]
    \centering
    \caption{\textbf{Evaluation of robustness and base to new generalizability.} We trained RPO and CoCoOp on 16-shot learning setting with 10 random seeds. mean denotes harmonic mean averaged over 10 random seeds and std denotes standard deviation of the 10 harmonic means.}
    \begin{tabular}{l@{\hspace{\tabcolsep}}cc@{\hspace{\tabcolsep}}cc@{\hspace{\tabcolsep}}cc@{\hspace{\tabcolsep}}cc@{\hspace{\tabcolsep}}cc@{\hspace{\tabcolsep}}cc@{\hspace{\tabcolsep}}cc}
        \toprule
        & \multicolumn{2}{c}{EuroSAT} & \multicolumn{2}{c}{FGVCAircraft}& \multicolumn{2}{c}{DTD} & \multicolumn{2}{c}{StanfordCars} & \multicolumn{2}{c}{UCF101} & \multicolumn{2}{c}{Flowers102}   \\
          \cmidrule(r){2-3}\cmidrule(r){4-5}\cmidrule(r){6-7}\cmidrule(r){8-9}\cmidrule(r){10-11}\cmidrule(r){12-13}\cmidrule(r){14-15} 
          &{CoCoOp} & {RPO} & {CoCoOP} & {RPO} & {CoCoOp} & {RPO} & {CoCoOp} & {RPO}& {CoCoOp} & {RPO}& {CoCoOp} & {RPO}\\
          \cmidrule(r){1-15}
        mean  & 73.65 & \textbf{74.38}  & 28.88 & \textbf{36.09} & 62.74 & \textbf{68.43} & 72.14 & \textbf{74.18} & 77.53& \textbf{79.75} & 81.42 & \textbf{84.23}\\
        std & 13.64 & \textbf{3.48} & 10.52 & \textbf{0.58} & 2.87 & \textbf{1.05} & 0.60 & \textbf{0.32} & 1.02 & \textbf{0.52} & 0.95 & \textbf{0.51}  \\
    \bottomrule
  \end{tabular}
  \label{tab:variance_analysis}
\end{table*}
