# Supplementary material for: Read-only Prompt Optimization for Vision-Language Few-shot Learning
Source: arXiv:2308.14960 source file (2023-11-10)
Supplement: Supplementary file 4 [file supple.tex]

% CVPR 2022 Paper Template
% based on the CVPR template provided by Ming-Ming Cheng (https://github.com/MCG-NKU/CVPR_Template)
% modified and extended by Stefan Roth (stefan.roth@NOSPAMtu-darmstadt.de)
\documentclass[10pt,twocolumn,letterpaper]{article}

%%%%%%%%% PAPER TYPE  - PLEASE UPDATE FOR FINAL VERSION
%\usepackage[review]{cvpr}      % To produce the REVIEW version
\usepackage{iccv}              % To produce the CAMERA-READY version
%\usepackage[pagenumbers]{iccv} % To force page numbers, e.g. for an arXiv version

% Include other packages here, before hyperref.
\usepackage{graphicx}
\usepackage{amsmath}
\usepackage{amssymb}
\usepackage{booktabs}
\usepackage{color, colortbl}
\usepackage{multirow}
\usepackage{subcaption}
\usepackage{pifont}% http://ctan.org/pkg/pifont

\definecolor{Gray}{gray}{0.9}
\definecolor{DarkGray}{gray}{0.5}

\usepackage{iccv}
\usepackage{times}
\usepackage{epsfig}
\usepackage{graphicx}
\usepackage{amsmath}
\usepackage{amssymb}
\usepackage{subcaption}
\usepackage{booktabs}
\usepackage{color, colortbl}
\usepackage{multirow}
\usepackage{pifont}% http://ctan.org/pkg/pifont

\definecolor{Gray}{gray}{0.9}
\definecolor{DarkGray}{gray}{0.5}

% Include other packages here, before hyperref.

% If you comment hyperref and then uncomment it, you should delete
% egpaper.aux before re-running latex.  (Or just hit 'q' on the first latex
% run, let it finish, and you should be clear).
\usepackage[pagebackref=true,breaklinks=true,letterpaper=true,colorlinks,bookmarks=false]{hyperref}
\iccvfinalcopy % *** Uncomment this line for the final submission

\usepackage[capitalize]{cleveref}
\pagenumbering{gobble}

% It is strongly recommended to use hyperref, especially for the review version.
% hyperref with option pagebackref eases the reviewers' job.
% Please disable hyperref *only* if you encounter grave issues, e.g. with the
% file validation for the camera-ready version.
%
% If you comment hyperref and then uncomment it, you should delete
% ReviewTempalte.aux before re-running LaTeX.
% (Or just hit 'q' on the first LaTeX run, let it finish, and you
%  should be clear).
%\usepackage[pagebackref,breaklinks,colorlinks]{hyperref}

% Support for easy cross-referencing
\usepackage[capitalize]{cleveref}
\crefname{section}{Sec.}{Secs.}
\Crefname{section}{Section}{Sections}
\Crefname{table}{Table}{Tables}
\crefname{table}{Tab.}{Tabs.}

%%%%%%%%% PAPER ID  - PLEASE UPDATE
 % *** Enter the CVPR Paper ID here

\begin{document}

%%%%%%%%% TITLE - PLEASE UPDATE
% For a paper whose authors are all at the same institution,
% omit the following lines up until the closing ``}''.
% Additional authors and addresses can be added with ``\and'',
% just like the second author.
% To save space, use either the email address or home page, not both
\title{Read-only Prompt Optimization for Vision-Language Few-shot Learning (Supplementary Materials)}
\maketitle

%%%%%%%%% BODY TEXT
\appendix
%\input{Tables/eurosat_typo}
%We first rectify the typo in Table 1.k of our main paper. The harmonic mean (H) of RPO on the EuroSAT benchmark will be updated as {\color{red}72.21 $\rightarrow$ 77.21} in our camera-ready version.

Here, we provide additional experiments and analyses which are not included in the main paper due to the limited space, which include ablation results of individual datasets and analysis about robustness of RPO on diverse benchmark datasets.

%%%%%%%%%%%%%%%%%%% ablation result for individual dataset %%%%%%%%%%%
\section {Ablation results on individual datasets}
In Section 4.3 of our main paper, we only provided averaged results due to limited space. Therefore, here we provide analysis results for each of the 11 image recognition datasets.

\subsection{Ablation on our components}
\begin{table*}[t]
  % \caption{\textbf{abbab.}
  % \centering
% \setlength{\tabcolsep}{6pt}
    % abcd
  % }
\caption{\textbf{Ablation on our components in base to new generalization setting.} We evaluate base to new generalization performance by ablating read-only mask and special initialization.}
  \begin{subtable}{0.3\linewidth}
  \centering
  \caption{Average over 11 datasets}
  \begin{tabular}{l|c|c|c}
    \toprule
    Methods & Base & Novel & H\\
    \midrule
    w.o mask & \textcolor{DarkGray}{79.97} & \textcolor{DarkGray}{69.90} & 74.02 \\
    w.o init & \textcolor{DarkGray}{82.27} & \textcolor{DarkGray}{72.78} & 76.78 \\
    RPO    &   \textcolor{DarkGray}{81.13}    &   \textcolor{DarkGray}{75.00}    &   \textbf{77.78} \\
    
    \bottomrule
    \end{tabular}
    \label{tab:9.a}
  \end{subtable}
  \hfill
  \begin{subtable}{0.3\linewidth}
  \centering
  \caption{ImageNet.}
  \begin{tabular}{l|c|c|c}
    \toprule
    Methods & Base & Novel & H\\
    \midrule
    w.o mask & \textcolor{DarkGray}{76.10} & \textcolor{DarkGray}{69.03} & 72.40 \\
    w.o init & \textcolor{DarkGray}{76.57} & \textcolor{DarkGray}{70.57} & 73.45 \\
    RPO    &   \textcolor{DarkGray}{76.60}    &   \textcolor{DarkGray}{71.57}    &   \textbf{74.00} \\
    
    \bottomrule
  \end{tabular}
  \label{tab:9.b}
  \end{subtable}
  \hfill
  \begin{subtable}{0.3\linewidth}
  \centering
  \caption{Caltech101.}
  \begin{tabular}{l|c|c|c}
    \toprule
    Methods & Base & Novel & H\\
    \midrule
    w.o mask & \textcolor{DarkGray}{98.10} & \textcolor{DarkGray}{92.87} & 95.41 \\
    w.o init & \textcolor{DarkGray}{98.60} & \textcolor{DarkGray}{92.47} & 95.43 \\
    RPO    &   \textcolor{DarkGray}{97.97}    &   \textcolor{DarkGray}{94.37}    &   \textbf{96.03} \\
    \bottomrule
  \end{tabular}
  \label{tab:9.c}
  \end{subtable}
  \hfill
  \vspace{0.5em}
  \begin{subtable}{0.3\linewidth}
  \centering
  \caption{OxfordPets.}
  \begin{tabular}{l|c|c|c}
    \toprule
    Methods & Base & Novel & H\\
    \midrule
    w.o mask & \textcolor{DarkGray}{95.13} & \textcolor{DarkGray}{96.77} & 95.95 \\
    w.o init & \textcolor{DarkGray}{95.57} & \textcolor{DarkGray}{96.90} & \textbf{96.23} \\
    RPO    &   \textcolor{DarkGray}{94.63}    &   \textcolor{DarkGray}{97.50}    &  96.05 \\
    \bottomrule
  \end{tabular}
  \label{tab:9.d}
  \end{subtable}
  \hfill
  \begin{subtable}{0.3\linewidth}
  \centering
  \caption{StanfordCars.}
  \begin{tabular}{l|c|c|c}
    \toprule
    Methods & Base & Novel & H\\
    \midrule
    w.o mask & \textcolor{DarkGray}{74.53} & \textcolor{DarkGray}{71.47} & 72.96 \\
    w.o init & \textcolor{DarkGray}{72.93} & \textcolor{DarkGray}{73.33} & 73.13 \\
    RPO    &   \textcolor{DarkGray}{73.87}    &   \textcolor{DarkGray}{75.53}    &   \textbf{74.69} \\
    \bottomrule
  \end{tabular}
  \label{tab:9.e}
  \end{subtable}
  \hfill
  \begin{subtable}{0.3\linewidth}
  \centering
  \caption{Flowers102.}
  \begin{tabular}{l|c|c|c}
    \toprule
    Methods & Base & Novel & H\\
    \midrule
    w.o mask & \textcolor{DarkGray}{96.87} & \textcolor{DarkGray}{71.47} & 82.92 \\
    w.o init & \textcolor{DarkGray}{94.70} & \textcolor{DarkGray}{74.83} & 83.60 \\
    RPO    &   \textcolor{DarkGray}{94.13}    &   \textcolor{DarkGray}{76.67}    &   \textbf{84.50} \\
    \bottomrule
  \end{tabular}
  \label{tab:9.f}
  \end{subtable}
  \hfill
  \vspace{0.5em}
  \begin{subtable}{0.3\linewidth}
  \centering
  \caption{Food101.}
  \begin{tabular}{l|c|c|c}
    \toprule
    Methods & Base & Novel & H\\
    \midrule
    w.o mask & \textcolor{DarkGray}{88.97} & \textcolor{DarkGray}{88.73} & 88.85 \\
    w.o init & \textcolor{DarkGray}{90.23} & \textcolor{DarkGray}{89.87} & 90.05 \\
    RPO    &   \textcolor{DarkGray}{90.33}    &   \textcolor{DarkGray}{90.83}    &   \textbf{90.58} \\
    \bottomrule
  \end{tabular}
  \label{tab:9.g}
  \end{subtable}
  \hfill
  \begin{subtable}{0.3\linewidth}
  \centering
  \caption{FGVCAircraft.}
  \begin{tabular}{l|c|c|c}
    \toprule
    Methods & Base & Novel & H\\
    \midrule
    w.o mask & \textcolor{DarkGray}{35.53} & \textcolor{DarkGray}{29.90} & 32.45 \\
    w.o init & \textcolor{DarkGray}{38.37} & \textcolor{DarkGray}{31.43} & 34.55 \\
    RPO    &   \textcolor{DarkGray}{37.33}    &   \textcolor{DarkGray}{34.20}    &   \textbf{35.70} \\
    \bottomrule
  \end{tabular}
  \label{tab:9.h}
  \end{subtable}
  \hfill
  \begin{subtable}{0.3\linewidth}
  \centering
  \caption{SUN397.}
  \begin{tabular}{l|c|c|c}
    \toprule
    Methods & Base & Novel & H\\
    \midrule
    w.o mask & \textcolor{DarkGray}{78.96} & \textcolor{DarkGray}{76.10} & 77.50 \\
    w.o init & \textcolor{DarkGray}{80.53} & \textcolor{DarkGray}{77.60} & 79.04 \\
    RPO    &   \textcolor{DarkGray}{80.60}    &   \textcolor{DarkGray}{77.80}    &   \textbf{79.18} \\
    \bottomrule
  \end{tabular}
  \label{tab:9.i}
  \end{subtable}
  \hfill
  \vspace{0.5em}
  \begin{subtable}{0.3\linewidth}
  \centering
  \caption{DTD.}
  \begin{tabular}{l|c|c|c}
    \toprule
    Methods & Base & Novel & H\\
    \midrule
    w.o mask & \textcolor{DarkGray}{78.67} & \textcolor{DarkGray}{55.77} & 65.25 \\
    w.o init & \textcolor{DarkGray}{79.93} & \textcolor{DarkGray}{63.13} & \textbf{70.53} \\
    RPO    &   \textcolor{DarkGray}{76.70}    &   \textcolor{DarkGray}{62.13}    &  68.61 \\
    \bottomrule
  \end{tabular}
  \label{tab:9.j}
  \end{subtable}
  \hfill
  \begin{subtable}{0.3\linewidth}
  \centering
  \caption{EuroSAT.}
  \begin{tabular}{l|c|c|c}
    \toprule
    Methods & Base & Novel & H\\
    \midrule
    w.o mask & \textcolor{DarkGray}{74.70} & \textcolor{DarkGray}{45.13} & 54.57 \\
    w.o init & \textcolor{DarkGray}{93.80} & \textcolor{DarkGray}{55.13} & 69.37 \\
    RPO    &   \textcolor{DarkGray}{86.63}    &   \textcolor{DarkGray}{68.97}    &   \textbf{76.79} \\
    \bottomrule
  \end{tabular}
  \label{tab:9.k}
  \end{subtable}
  \hfill
  \vspace{0.5em}
  \begin{subtable}{0.3\linewidth}
  \centering
  \caption{UCF101.}
  \begin{tabular}{l|c|c|c}
    \toprule
    Methods & Base & Novel & H\\
    \midrule
    w.o mask & \textcolor{DarkGray}{82.07} & \textcolor{DarkGray}{70.63} & 75.92 \\
    w.o init & \textcolor{DarkGray}{83.77} & \textcolor{DarkGray}{75.27} & 79.29 \\
    RPO    &   \textcolor{DarkGray}{83.67}    &   \textcolor{DarkGray}{75.43}    &   \textbf{79.34} \\
    \bottomrule
  \end{tabular}
  \label{tab:9.l}
  \end{subtable}
  \hfill
  \vspace{0.5em}
\label{tab:ablation_11}
\end{table*} 

\begin{table*}[h]
  % \caption{\textbf{abbab.}
  % \centering
% \setlength{\tabcolsep}{6pt}
    % abcd
  % }
\caption{\textbf{Comparison of CoCoOp, vis-RPO, text-RPO and RPO in the Base to new generalization setting.} We evaluate base to new generalization performance with unimodal RPO trained with 16-shot sampled training data.}
  \begin{subtable}{0.3\linewidth}
  \centering
  \caption{Average over 11 datasets}
  \begin{tabular}{l|c|c|c}
    \toprule
    Methods & Base & Novel & H\\
    \midrule
    CoCoOp  &   \textcolor{DarkGray}{80.47}   &   \textcolor{DarkGray}{71.69}   &  75.83  \\
    \midrule
    text-RPO & \textcolor{DarkGray}{79.54} & \textcolor{DarkGray}{74.83} & 77.01 \\
    RPO    &   \textcolor{DarkGray}{81.13}    &   \textcolor{DarkGray}{75.00}    &   \textbf{77.78} \\
    \bottomrule
    \end{tabular}
    \label{tab:11.a}
  \end{subtable}
  \hfill
  \begin{subtable}{0.3\linewidth}
  \centering
  \caption{ImageNet.}
  \begin{tabular}{l|c|c|c}
    \toprule
    Methods & Base & Novel & H\\
    \midrule
    CoCoOp  &   \textcolor{DarkGray}{75.98}   &   \textcolor{DarkGray}{70.43}   &   73.10 \\
    \midrule
    text-RPO & \textcolor{DarkGray}{76.13} & \textcolor{DarkGray}{70.70} & 73.31 \\
    RPO    &   \textcolor{DarkGray}{76.60}    &   \textcolor{DarkGray}{71.57}    &   \textbf{74.00} \\
    \bottomrule
  \end{tabular}
  \label{tab:11.b}
  \end{subtable}
  \hfill
  \begin{subtable}{0.3\linewidth}
  \centering
  \caption{Caltech101.}
  \begin{tabular}{l|c|c|c}
    \toprule
    Methods & Base & Novel & H\\
    \midrule
    CoCoOp  &   \textcolor{DarkGray}{97.96}   &   \textcolor{DarkGray}{93.81}   &  95.84  \\
    \midrule
    text-RPO & \textcolor{DarkGray}{97.76} & \textcolor{DarkGray}{93.96} & 95.82 \\
    RPO    &   \textcolor{DarkGray}{97.97}    &   \textcolor{DarkGray}{94.37}    &  \textbf{96.03}  \\
    \bottomrule
  \end{tabular}
  \label{tab:11.c}
  \end{subtable}
  \hfill
  \vspace{0.5em}
  \begin{subtable}{0.3\linewidth}
  \centering
  \caption{OxfordPets.}
  \begin{tabular}{l|c|c|c}
    \toprule
    Methods & Base & Novel & H\\
    \midrule
    CoCoOp  &   \textcolor{DarkGray}{95.20}   &   \textcolor{DarkGray}{97.69}   &  \textbf{96.43} \\
    \midrule
    text-RPO & \textcolor{DarkGray}{94.56} & \textcolor{DarkGray}{97.16} & 95.84 \\
    RPO    &   \textcolor{DarkGray}{94.63}    &   \textcolor{DarkGray}{97.50}    &   96.05 \\
    \bottomrule
  \end{tabular}
  \label{tab:11.d}
  \end{subtable}
  \hfill
  \begin{subtable}{0.3\linewidth}
  \centering
  \caption{StanfordCars.}
  \begin{tabular}{l|c|c|c}
    \toprule
    Methods & Base & Novel & H \\
    \midrule
    CoCoOp  &   \textcolor{DarkGray}{70.49}  &   \textcolor{DarkGray}{73.59}   &   72.01 \\
    \midrule
    text-RPO & \textcolor{DarkGray}{72.16} & \textcolor{DarkGray}{74.4} & 73.26 \\
    RPO    &   \textcolor{DarkGray}{73.87}    &   \textcolor{DarkGray}{75.53}    &  \textbf{74.69}  \\
    \bottomrule
  \end{tabular}
  \label{tab:11.e}
  \end{subtable}
  \hfill
  \begin{subtable}{0.3\linewidth}
  \centering
  \caption{Flowers102.}
  \begin{tabular}{l|c|c|c}
    \toprule
    Methods & Base & Novel & H\\
    \midrule
    CoCoOp  &   \textcolor{DarkGray}{94.87}   &   \textcolor{DarkGray}{71.75}   &   81.71 \\
    \midrule
    text-RPO & \textcolor{DarkGray}{91.70} & \textcolor{DarkGray}{74.90} & 82.45 \\
    RPO    &   \textcolor{DarkGray}{94.13}    &   \textcolor{DarkGray}{76.67}    &   \textbf{84.50} \\
    \bottomrule
  \end{tabular}
  \label{tab:11.f}
  \end{subtable}
  \hfill
  \vspace{0.5em}
  \begin{subtable}{0.3\linewidth}
  \centering
  \caption{Food101.}
  \begin{tabular}{l|c|c|c}
    \toprule
    Methods & Base & Novel & H\\
    \midrule
    CoCoOp  &   \textcolor{DarkGray}{90.70}   &   \textcolor{DarkGray}{91.29}   &   \textbf{90.99} \\
    \midrule
    text-RPO & \textcolor{DarkGray}{89.90} & \textcolor{DarkGray}{90.06} & 89.98 \\
    RPO    &   \textcolor{DarkGray}{90.33}    &   \textcolor{DarkGray}{90.83}    &   90.58
 \\
    \bottomrule
  \end{tabular}
  \label{tab:11.g}
  \end{subtable}
  \hfill
  \begin{subtable}{0.3\linewidth}
  \centering
  \caption{FGVCAircraft.}
  \begin{tabular}{l|c|c|c}
    \toprule
    Methods & Base & Novel & H\\
    \midrule
    CoCoOp  &   \textcolor{DarkGray}{33.41}   &   \textcolor{DarkGray}{23.71}   &   27.74 \\
    \midrule
    text-RPO & \textcolor{DarkGray}{36.5} & \textcolor{DarkGray}{35.7} & \textbf{36.09} \\
    RPO    &   \textcolor{DarkGray}{37.33}    &   \textcolor{DarkGray}{34.20}    &  35.70  \\
    \bottomrule
  \end{tabular}
  \label{tab:11.h}
  \end{subtable}
  \hfill
  \begin{subtable}{0.3\linewidth}
  \centering
  \caption{SUN397.}
  \begin{tabular}{l|c|c|c}
    \toprule
    Methods & Base & Novel & H\\
    \midrule
    CoCoOp  &   \textcolor{DarkGray}{79.74}   &   \textcolor{DarkGray}{76.86}   &   78.27 \\
    \midrule
    text-RPO & \textcolor{DarkGray}{79.56} & \textcolor{DarkGray}{77.03} & 78.27 \\
    RPO    &   \textcolor{DarkGray}{80.60}    &   \textcolor{DarkGray}{77.80}    &   \textbf{79.18} \\
    \bottomrule
  \end{tabular}
  \label{tab:11.i}
  \end{subtable}
  \hfill
  \vspace{0.5em}
  \begin{subtable}{0.3\linewidth}
  \centering
  \caption{DTD.}
  \begin{tabular}{l|c|c|c}
    \toprule
    Methods & Base & Novel & H\\
    \midrule
    CoCoOp  &   \textcolor{DarkGray}{77.01}   &   \textcolor{DarkGray}{56.00}   &   64.85 \\
    \midrule
    text-RPO & \textcolor{DarkGray}{75.06} & \textcolor{DarkGray}{62.60} & 68.26 \\
    RPO    &   \textcolor{DarkGray}{76.70}    &   \textcolor{DarkGray}{62.13}    &  \textbf{68.61} \\
    \bottomrule
  \end{tabular}
  \label{tab:11.j}
  \end{subtable}
  \hfill
  \begin{subtable}{0.3\linewidth}
  \centering
  \caption{EuroSAT.}
  \begin{tabular}{l|c|c|c}
    \toprule
    Methods & Base & Novel & H\\
    \midrule
    CoCoOp  &   \textcolor{DarkGray}{87.49}   &   \textcolor{DarkGray}{60.04}   &   71.21 \\
    \midrule
    text-RPO & \textcolor{DarkGray}{79.90} & \textcolor{DarkGray}{71.60} & 75.52 \\
    RPO    &   \textcolor{DarkGray}{86.63}    &   \textcolor{DarkGray}{68.97}    &   \textbf{76.79} \\
    \bottomrule
  \end{tabular}
  \label{tab:11.k}
  \end{subtable}
  \hfill
  %\vspace{0.5em}
  \begin{subtable}{0.3\linewidth}
  \centering
  \caption{UCF101.}
  \begin{tabular}{l|c|c|c}
    \toprule
    Methods & Base & Novel & H\\
    \midrule
    CoCoOp  &   \textcolor{DarkGray}{82.33}   &   \textcolor{DarkGray}{73.45}   &   77.64 \\
    \midrule
    text-RPO & \textcolor{DarkGray}{81.70} & \textcolor{DarkGray}{75.1} & 78.26 \\
    RPO    &   \textcolor{DarkGray}{83.67}    &   \textcolor{DarkGray}{75.43}    &   \textbf{79.34} \\
    \bottomrule
  \end{tabular}
  \label{tab:11.l}
  \end{subtable}
  \hfill
  \vspace{0.5em}
\label{tab:uni_rpo_11}
\end{table*}

\textbf{Ablation on read-only mask}
As shown in \Cref{tab:ablation_11}, removing the read-only mask results in a drop of generalization performance on 10 out of 11 datasets based on the harmonic mean of base and novel accuracy. Additionally, novel accuracy deteriorates on all datasets without masked attention, which supports our claim that the read-only mechanism aids generalization. \\

\textbf{Ablation on initialization}
Omitting the proposed initialization results in the improvement of `base' accuracy and the loss of `novel' accuracy on 7 out of 11 datasets. 
It shows worse generalization performance (evaluated by harmonic mean) on 9 out of 11 datasets. 
We believe that initializing prompts with pre-trained special tokens enables converging to a hypothesis with better generalizability.

\subsection{Ablation on multi-modality of prompt}
To show that the performance boost of RPO is not due to the multi-modality of prompts but the read-only mechanism, we provide the base-to-new generalization performance of RPO with only learnable text prompts (text-RPO). For text-RPO, we exploit global image feature of pre-trained ViT-B/16 backbone as image feature.\\

\textbf{RPO with only learnable text prompts}
As shown in \Cref{tab:uni_rpo_11}, text-RPO results in a marginal performance drop (0.8\%) compared to RPO on average. To be specific, text-RPO even outperforms RPO on FGVCAircraft datasets by a small margin. Addtionally, text-RPO outperforms CoCoOp on 8 out of 11 datasets, which supports the effectiveness of read-only mechanism compared to conventional prompt tuning.\\

\end{document}
